# Supplementary material for: Curl-Flow: Boundary-Respecting Pointwise Incompressible Velocity Interpolation for Grid-Based Fluids
Source: arXiv:2104.00867 source file (2023-11-26)
Supplement: Supplementary file 1 [file 8.appendix.tex]

\section{Bilinear velocity interpolation is divergent}
\label{app:bilinear}

To see the problem with standard interpolants, define a linear interpolation function $lerp(a,b,t)= (1-t)a+t b$ and construct the bilinearly interpolated velocity at a point $P=(x,y)$ (see Figure~\ref{fig:velocityInterpolation}) as
\begin{equation}
\label{eq:velocityInterpolation} 
\begin{aligned}
u(x, y) &= lerp(lerp(u_0,u_1, \alpha_u(x)), lerp(u_2,u_3, \alpha_u(x)), \beta_u(y)) \\
v(x,y) &=  lerp(lerp(v_0,v_1, \alpha_v(x)), lerp(v_2,v_3, \alpha_v(x)), \beta_v(y)) 
\end{aligned}
\end{equation}
where the ${\alpha}$ and ${\beta}$ functions return edge fractions (${ 0 \leq \alpha, \beta \leq 1 }$) for the data indicated by their subscripts.
This interpolated velocity is not analytically divergence-free in general:
\begin{equation}
\label{eq:velocityInterpolationDivergence} 
\begin{aligned}
\nabla \cdot \mathbf{u} &= \frac{lerp(u_1-u_0, u_3-u_2, \beta_u(y))+lerp(v_2-v_0, v_3-v_1, \alpha_v(x))}{h}\\
& \neq 0
\end{aligned}
\end{equation}
The grid cell width $h$ appears due to the derivatives of $\alpha$ and $\beta$.

\begin{figure}
\begin{overpic}[width=2.5in]{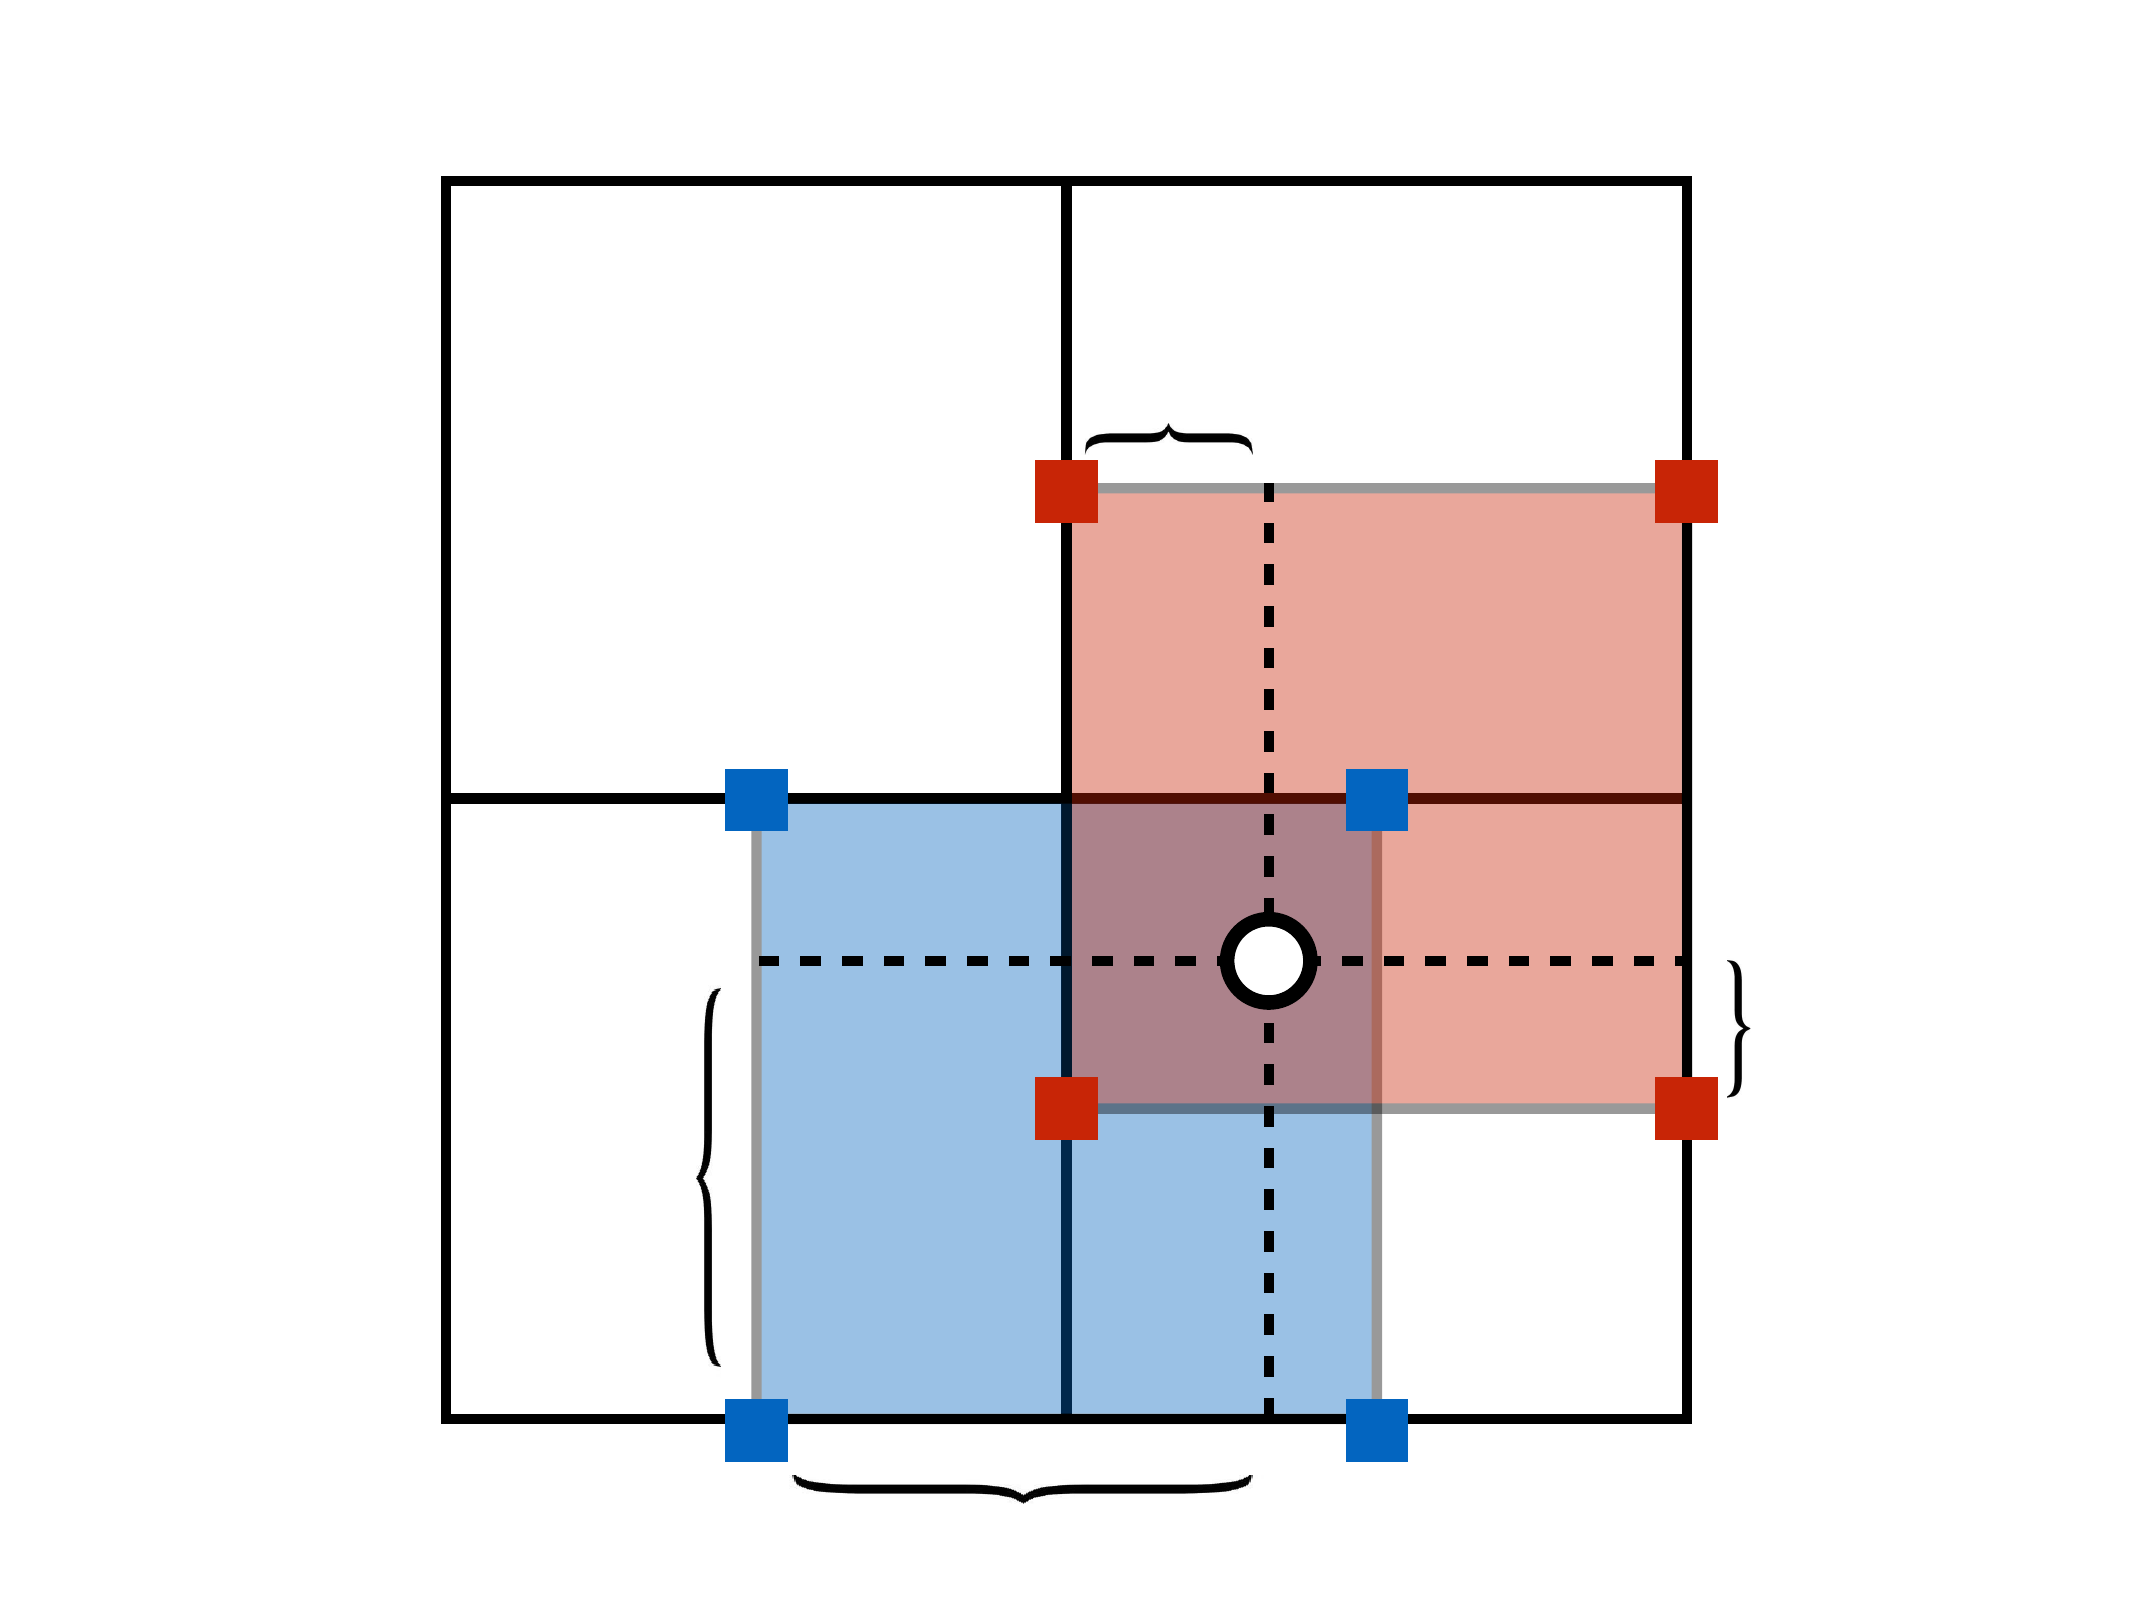}
\put(42, 21) { ${ u_0}$ }
\put(42, 52) { ${ u_2}$ }
\put(82, 21) { ${ u_1}$ }
\put(82, 52) { ${ u_3}$ }

\put(50, 57) { ${ \alpha_u}$ }
\put(82, 26) { ${ \beta_u}$ }

\put(28, 3) { ${ v_0}$ }
\put(28, 34) { ${ v_2}$ }
\put(66, 3) { ${ v_1}$ }
\put(66, 34) { ${ v_3}$ }

\put(46.5, 1) { ${ \alpha_v }$ }
\put(25.5, 18.5) { ${ \beta_v }$ }

\put(60, 24.5) { ${ P }$ }

\end{overpic}
\caption{\textbf{Direct Velocity Interpolation:} 
To compute a pointwise velocity at point $P = (x,y)$ in a staggered velocity grid,
 one (bilinearly) interpolates the nearby velocity samples component by component. }
\label{fig:velocityInterpolation}
\end{figure}

\section{Curl-Flow Ramp in 3D}
\label{app:curlFlowRamp}
Defining ${r = \frac{|| \mathbf{x} - \textbf{cp}(\mathbf{x}) ||}{h}}$, the terms in 
\eqref{eq:modifiedVelocity3D} can be derived as:
\begin{equation}
\begin{aligned}
\nabla \times \boldsymbol{\psi}_{tan}(\textbf{cp}(\mathbf{x})) &=
\nabla \times \{\boldsymbol{\psi}(\textbf{cp}(\mathbf{x})) -
(\boldsymbol{\psi}(\textbf{cp}(\mathbf{x})) \cdot \mathbf{n}) \ \mathbf{n}\} \\
&=
\nabla \times \boldsymbol{\psi}(\textbf{cp}(\mathbf{x})) -
(\mathbf{n}\cdot \nabla)\boldsymbol{\psi}(\textbf{cp}(\mathbf{x})) \times \mathbf{n} \\
\nabla \times \boldsymbol{\psi}(\textbf{cp}(\mathbf{x})) &=
\frac{\partial \textbf{cp}(\mathbf{x})}{\partial \mathbf{x}}
\frac{\partial}{\partial \textbf{cp}(\mathbf{x})}
\times \boldsymbol{\psi}(\textbf{cp}(\mathbf{x})) \\
\nabla \times \boldsymbol{\psi}_{g, tan}(\textbf{cp}(\mathbf{x})) &=
\frac{\partial \textbf{cp}(\mathbf{x})}{\partial \mathbf{x}}
\frac{\partial}{\partial \textbf{cp}(\mathbf{x})}
\times \boldsymbol{\psi_{g, tan}}(\textbf{cp}(\mathbf{x})) \\
\frac{\partial \alpha(\mathbf{x}, \textbf{cp}(\mathbf{x}))}{\partial \mathbf{x}} &=
\frac{\partial \ {ramp(r)} }{\partial r} \frac{1}{h} 
\frac{\partial (\mathbf{x} - \textbf{cp}(\mathbf{x}))}{\partial \mathbf{x}}
\frac{\mathbf{x} - \textbf{cp}(\mathbf{x})}{||\mathbf{x} - \textbf{cp}(\mathbf{x})||} \\
\frac{\partial \psi(\textbf{cp}(\mathbf{x}))}{\partial \mathbf{x}} &=
\frac{\partial \textbf{cp}(\mathbf{x})}{\partial \mathbf{x}} \frac{\partial \psi(\textbf{cp}(\mathbf{x}))}{\partial \textbf{cp}(\mathbf{x})}
\end{aligned}
\end{equation}
